# Supplementary material for: Extending Attack Graphs to Represent Cyber-Attacks in Communication Protocols and Modern IT Networks
Source: arXiv:1906.09786 source file (2019-06-24)
Supplement: Supplementary file 1 [file attackGraphs.tex]

\subsection{\label{app:bus-spoof-poc}Bus Spoofing}
    \input{attack-graphs/bus_spoof}

\twocolumn
\subsection{\label{app:mitm-poc}Man-in-the-Middle}
    \input{attack-graphs/mitm}
    
\subsection{\label{app:dns-spoof-poc}DNS Spoofing}
    \input{attack-graphs/dns_spoof}

\newpage    
\subsection{\label{app:syn-flood-poc}SYN Flooding}
    \input{attack-graphs/syn_flood}

\subsection{\label{app:pin-crack-poc}Bluetooth PIN Cracking}
    \input{attack-graphs/pin_crack}
    
\newpage
\subsection{\label{app:wep-crack-poc}WEP Cracking}
    \input{attack-graphs/wep_crack}
    
\subsection{\label{app:bus-dos-poc}Bus Denial of Service}
    \input{attack-graphs/bus_dos}
